# Supplementary material for: X-Adapter: Adding Universal Compatibility of Plugins for Upgraded Diffusion Model
Source: arXiv:2312.02238 source file (2024-04-23)
Supplement: Supplementary file 2 [file supp_controlnet_tile.tex]

\begin{figure}[t]
    \centering
    \includegraphics[width=\columnwidth]{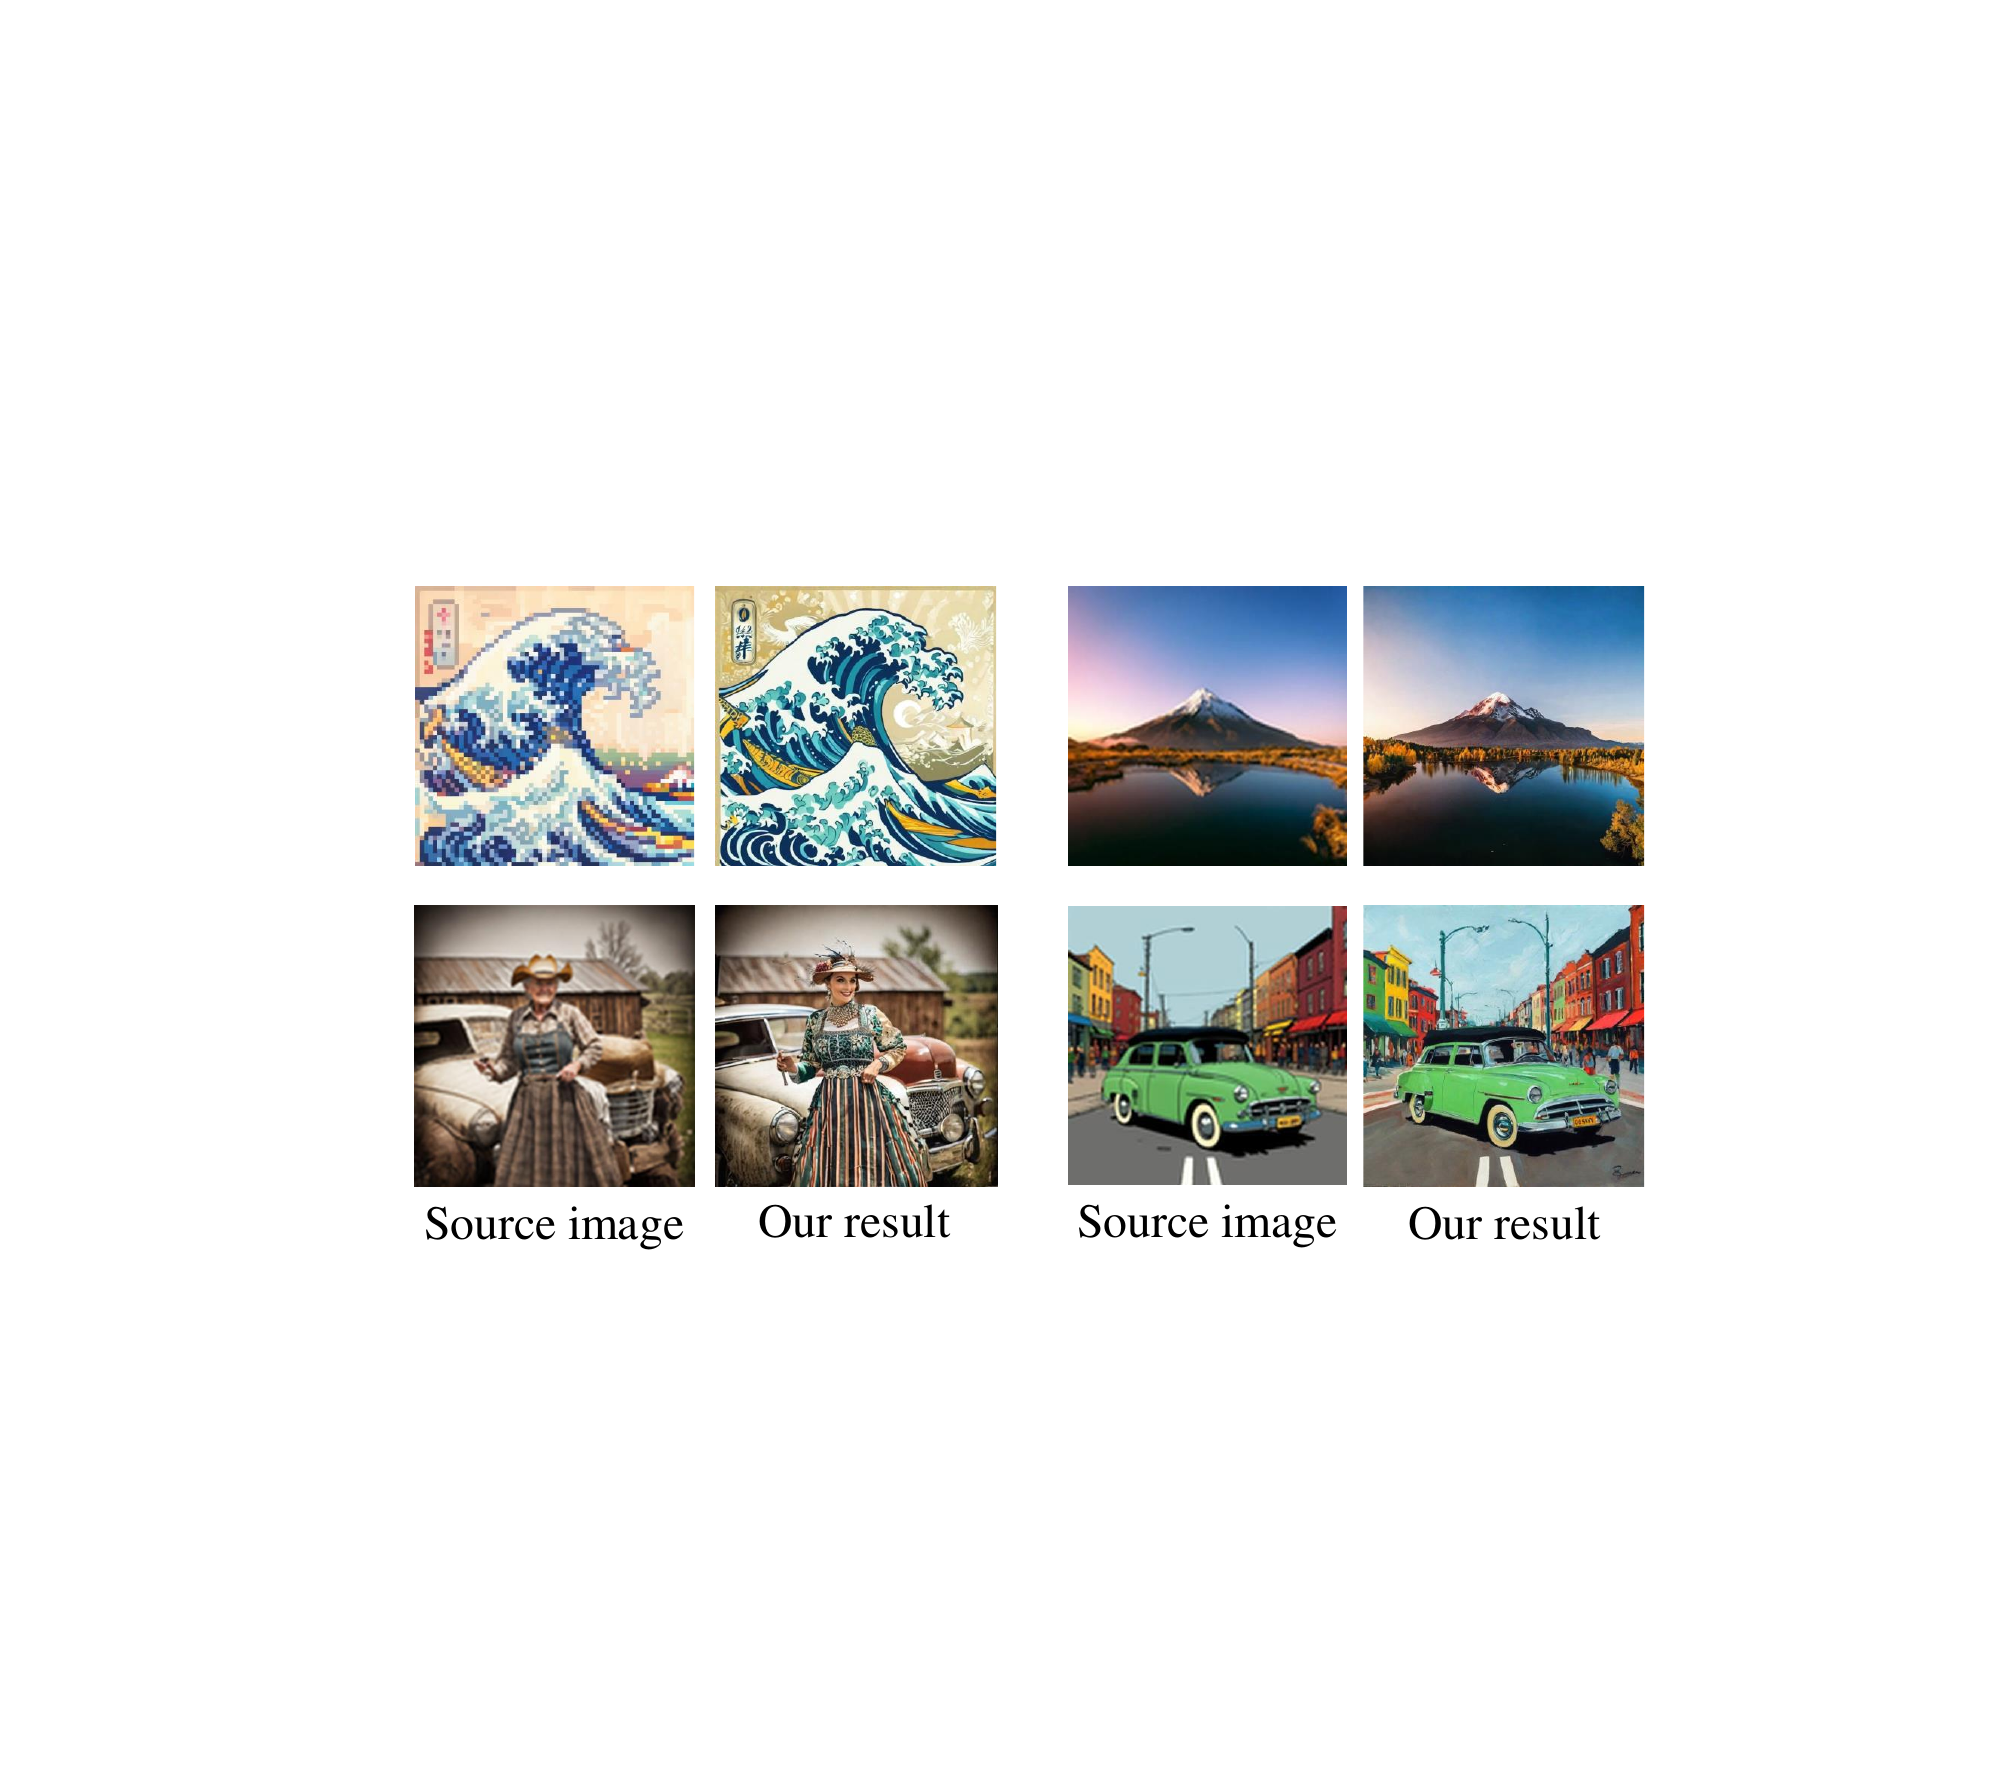}
    \vspace{-1.5em}
    \caption{ \textit{\textbf{Qualitative result on Controlnet-Tile}}. 
}
    \label{fig:Controlnet_tile_Supp}
\end{figure}
