# Supplementary material for: X-Adapter: Adding Universal Compatibility of Plugins for Upgraded Diffusion Model
Source: arXiv:2312.02238 source file (2024-04-23)
Supplement: Supplementary file 3 [file supp_lora.tex]

\begin{figure}[t]
    \centering
    \includegraphics[width=\columnwidth]{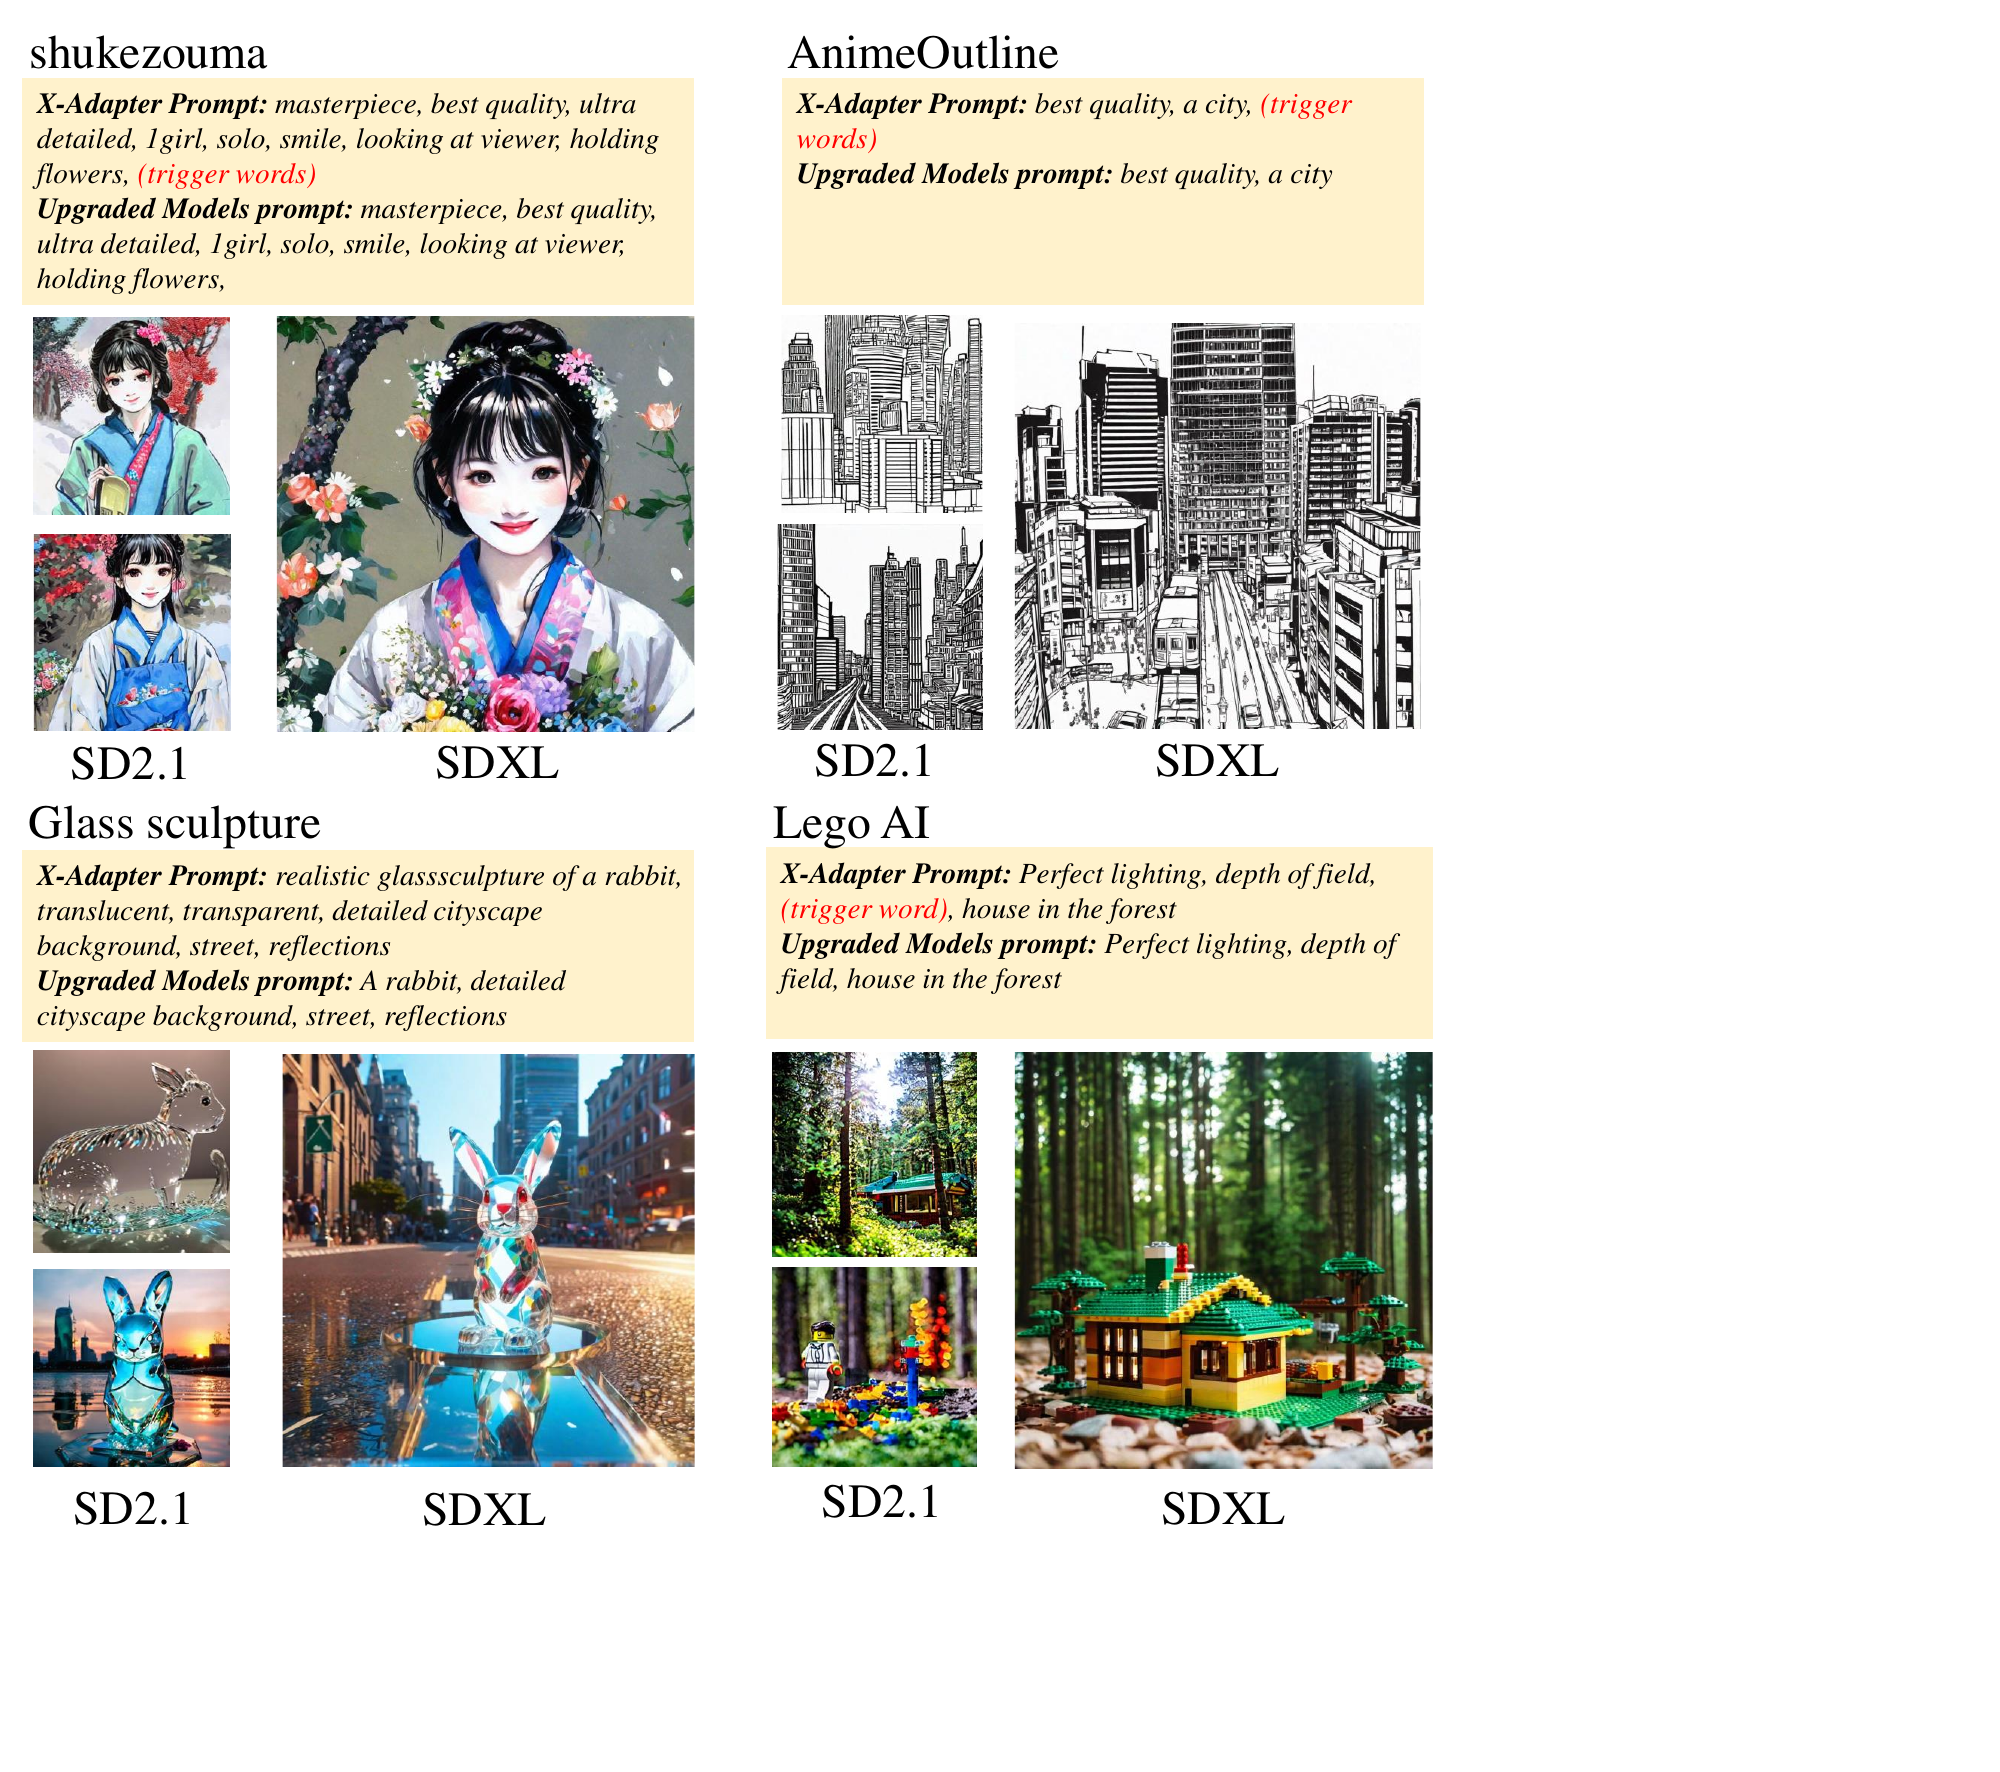}
    \vspace{-1.5em}
    \caption{ \textit{\textbf{Qualitative result on LoRA}}. 
}
    \label{fig:LoRA_Supp}
    \vspace{-1.20em}
\end{figure}
